# Supplementary material for: Towards Model Generalization for Monocular 3D Object Detection
Source: arXiv:2205.11664 source file (2022-06-13)
Supplement: Supplementary file 1 [file appendix.tex]

\appendix
\section{Appendix}

Optionally include extra information (complete proofs, additional experiments and plots) in the appendix.
This section will often be part of the supplemental material.
